# Supplementary material for: Powers of layers for image-to-image translation
Source: arXiv:2008.05763 source file (2020-08-13)
Supplement: Supplementary file 1 [file appendix_figure3.tex]

\begin{figure*}
\centering
\small
\begin{tabular}{cccc}
 Photo $\rightarrow$ Van Gogh & Photo $\rightarrow$ Monet & Zebra $\rightarrow$ Horse & Horse $\rightarrow$ Zebra \\
 \includegraphics[width=0.25\linewidth]{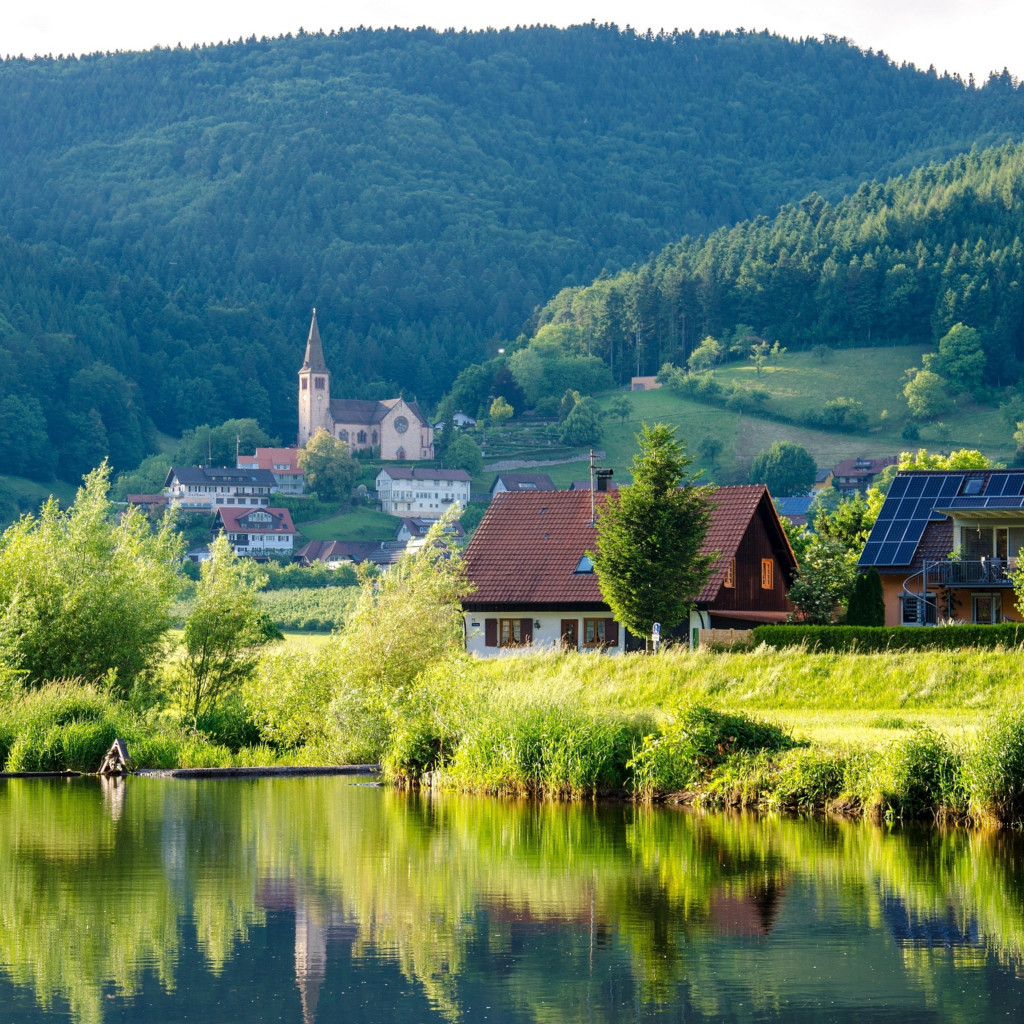}&
 \includegraphics[width=0.25\linewidth]{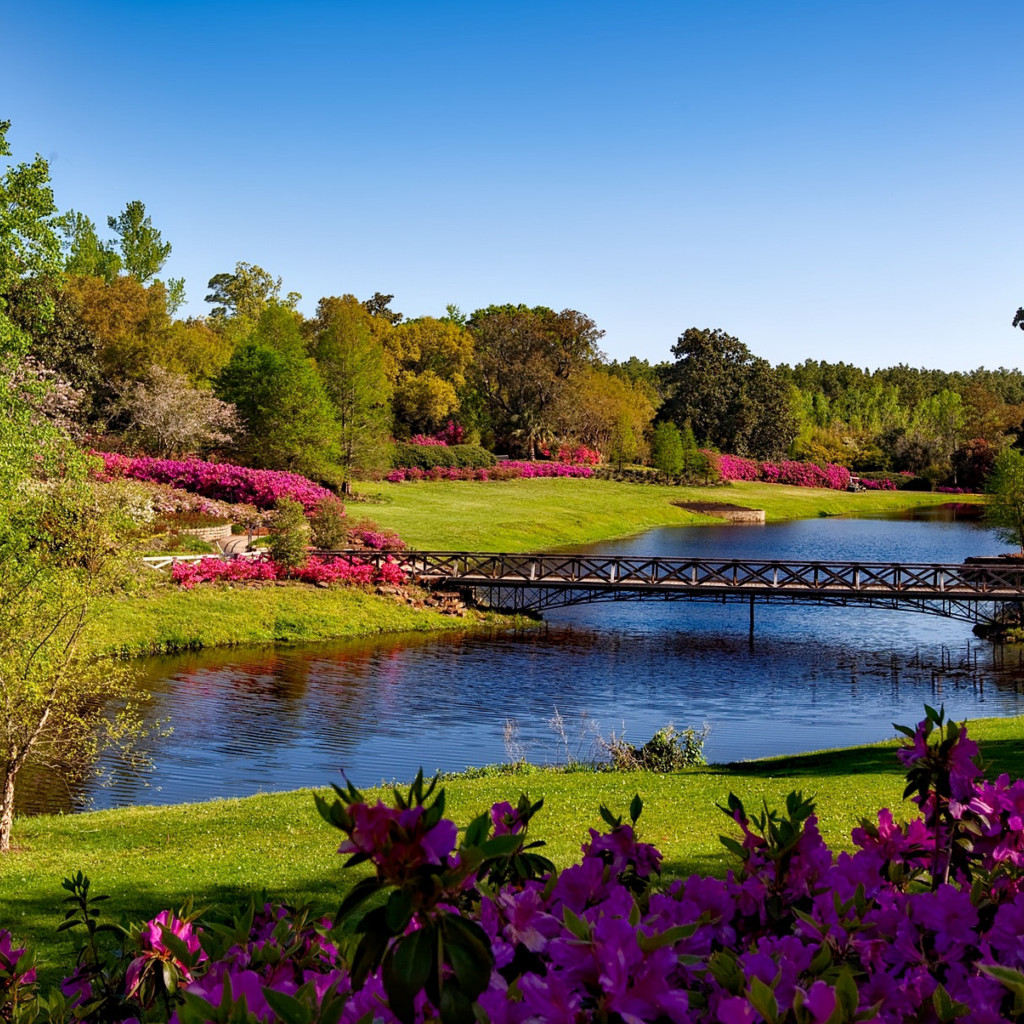}&
  \includegraphics[width=0.25\linewidth]{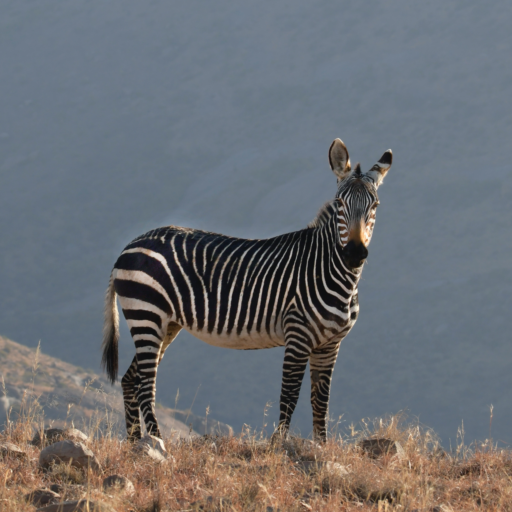}
   &\includegraphics[width=0.25\linewidth]{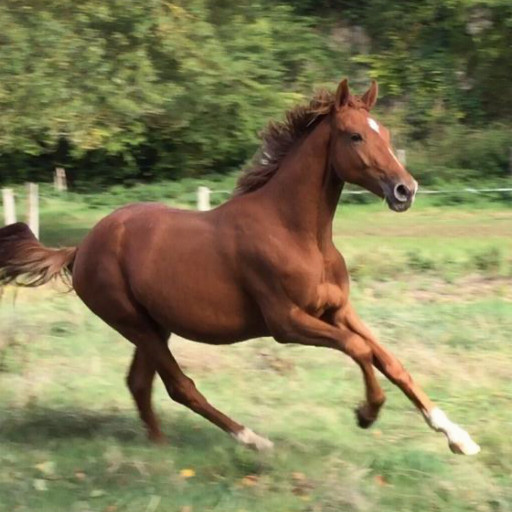}\\
  \includegraphics[width=0.25\linewidth]{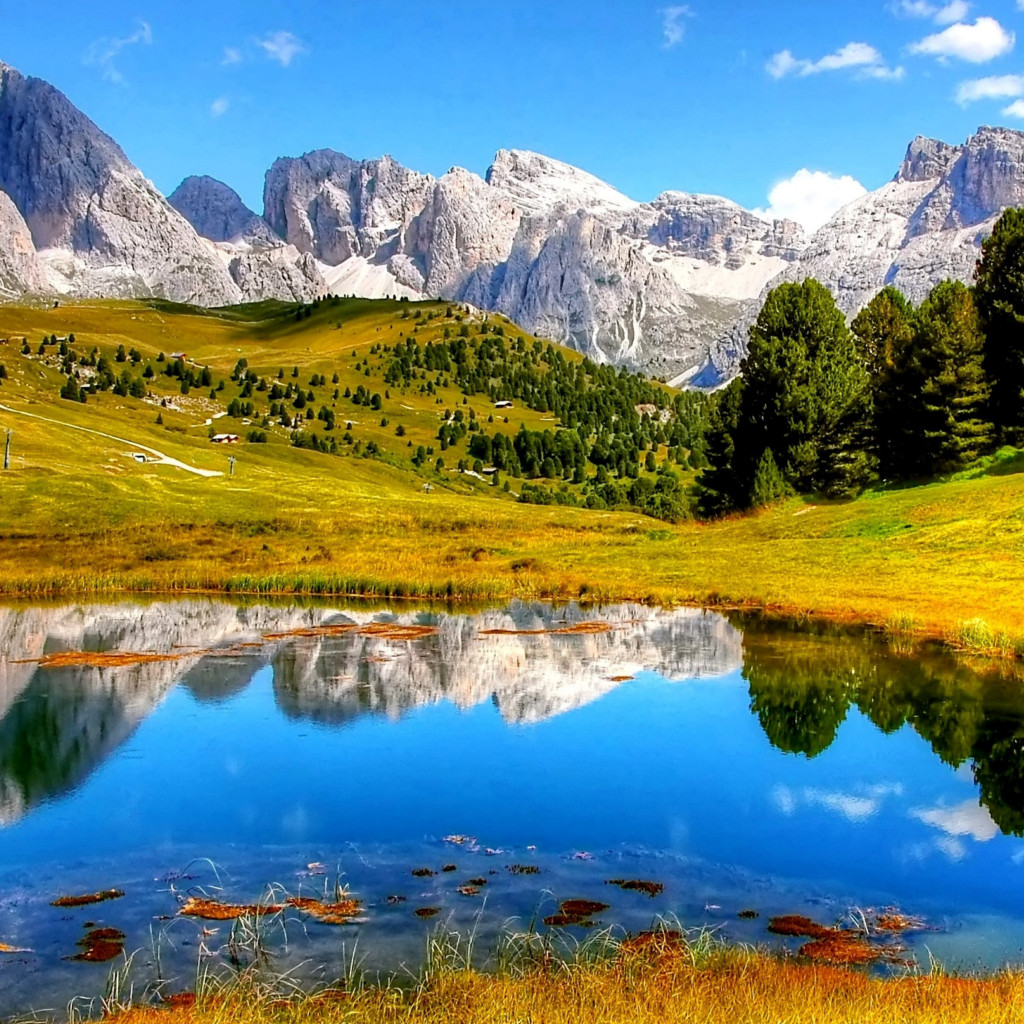}
  &\includegraphics[width=0.25\linewidth]{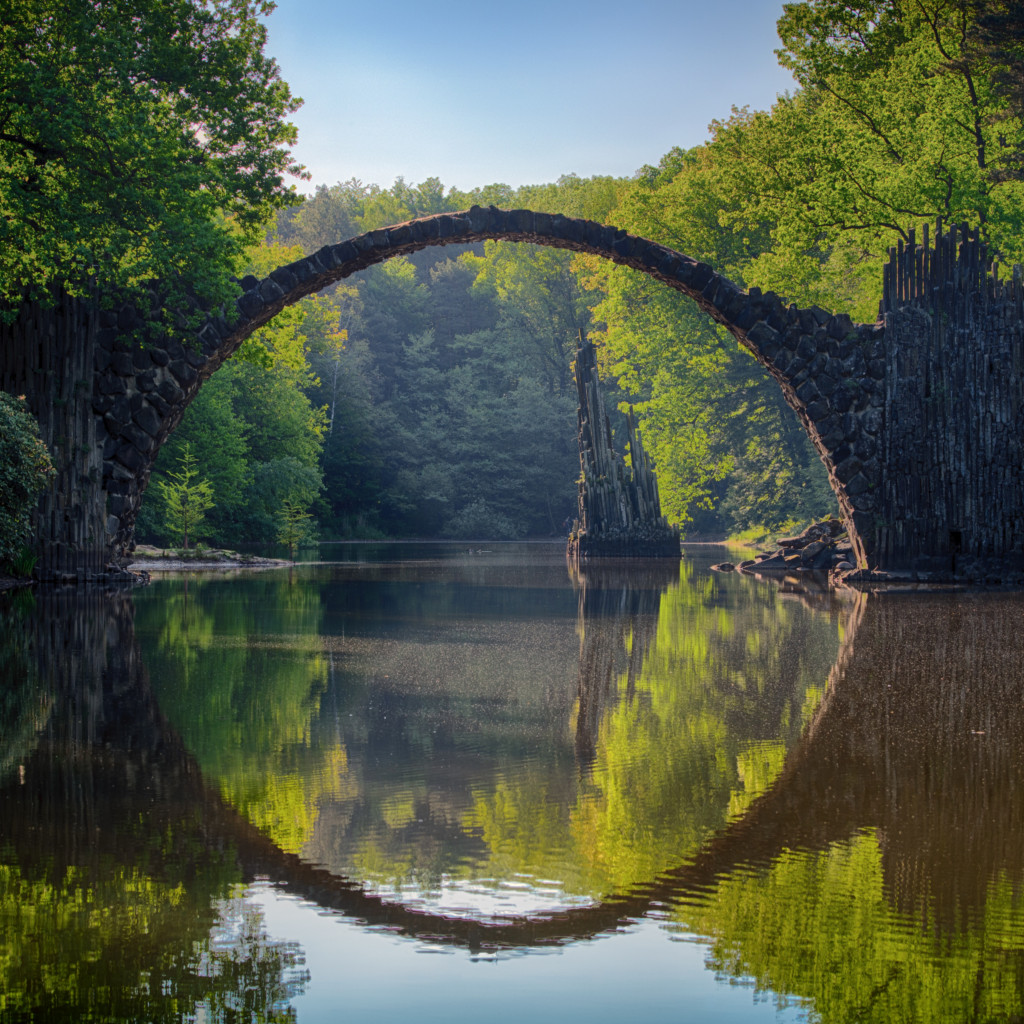}&  \includegraphics[width=0.25\linewidth]{images/High_Resolution/Zebra/im_zebra_org_6.png}
  &\includegraphics[width=0.25\linewidth]{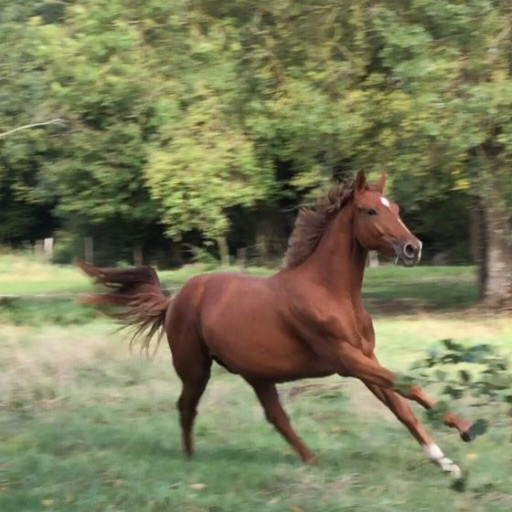}\\
\end{tabular}
\caption{\label{fig:org_highres}
Original images of figure~\ref{fig:highres}
}
\vspace{-1em}
\end{figure*}
